# Supplementary material for: Globally-Optimal Inlier Set Maximisation for Simultaneous Camera Pose and Feature Correspondence
Source: arXiv:1709.09384 ancillary file (2017-09-27)
Supplement: Supplementary file 1 [file appendix.pdf]

# APPENDIX

## A. Rotation Uncertainty Angle: Implementation Details

Lemma 3, copied below, requires the evaluation of $\max_{\mathbf{r}\in\mathcal{S}_r} \angle(\mathtt{R}_\mathbf{r}\mathbf{p}, \mathtt{R}_{\mathbf{r}_0}\mathbf{p})$, where $\mathbf{p}$ is any 3D point, $\mathbf{r}_0$ is the angle-axis vector at the centre of rotation cube $\mathcal{C}_r$ with surface $\mathcal{S}_r$ and $\mathtt{R}_\mathbf{r}$ is the rotation matrix induced by angle-axis vector $\mathbf{r}$.

**Lemma 3.** *(Rotation uncertainty angle) Given a 3D point* $\mathbf{p}$ *and a rotation cube* $\mathcal{C}_r$ *centred at* $\mathbf{r}_0$ *with surface* $\mathcal{S}_r$*, then* $\forall \mathbf{r} \in \mathcal{C}_r$*,*

$$\angle(\mathtt{R}_\mathbf{r}\mathbf{p}, \mathtt{R}_{\mathbf{r}_0}\mathbf{p}) \leqslant \min(\max_{\mathbf{r}\in\mathcal{S}_r} \angle(\mathtt{R}_\mathbf{r}\mathbf{p}, \mathtt{R}_{\mathbf{r}_0}\mathbf{p}), \pi) \triangleq \psi_r(\mathbf{p}, \mathcal{C}_r). \tag{1}$$

*Proof.* Inequality (1) can be derived as follows:

$$\angle(\mathtt{R}_\mathbf{r}\mathbf{p}, \mathtt{R}_{\mathbf{r}_0}\mathbf{p}) \leqslant \min(\max_{\mathbf{r}\in\mathcal{C}_r} \angle(\mathtt{R}_\mathbf{r}\mathbf{p}, \mathtt{R}_{\mathbf{r}_0}\mathbf{p}), \pi) \tag{2}$$

$$= \min(\max_{\mathbf{r}\in\mathcal{S}_r} \angle(\mathtt{R}_\mathbf{r}\mathbf{p}, \mathtt{R}_{\mathbf{r}_0}\mathbf{p}), \pi) \tag{3}$$

where (3) is a consequence of the order-preserving mapping, with respect to the radial angle, from the convex cube of angle-axis vectors to the spherical surface patch, since the mapping is obtained by projecting from the centre of the sphere to the surface of the sphere. □

While it is possible to calculate the bound by sampling the cube surface using a grid of step-size $\sigma_g$, evaluating the angle at each sample and adding $\sqrt{2}/2 \times \sigma_g$ to the greatest angle calculated (by Lemma 1), it is significantly more computationally efficient to use a different approach. We make two assumptions: (i) the maximum always occurs on the cube skeleton (edges and vertices), not the faces; and (ii) the angle function along each edge is quasiconvex or concave (specifically unimodal). The former assumption (i) has been demonstrated empirically in simulations and can be seen in Figure A.1, where it can be observed that rotation vectors on the cube faces are not projected beyond the convex hull of the projection of the edges for a given point. Therefore, the projected angle maximiser can always be found on an edge or vertex. The latter assumption (ii) has also been demonstrated empirically in simulations for all rotation cubes used in the GOPAC algorithm (that is, octree subdivisions of the angle-axis cube $[-\pi, \pi]^3$). In the vast majority of cases, the function is (quasi)convex, meaning that the angle maximiser occurs at one of the two vertices joined by the edge (the extreme points). In a small fraction of cases, the maximum occurs on the edge, but not at a vertex, as in Figure A.1. In these cases the assumption of unimodality allows us to use an efficient search routine, golden section search, which does not require the time-consuming evaluation of the derivative.

Our approach for calculating the rotation uncertainty angle $\psi_r(\mathbf{f}, \mathcal{C}_r)$ for a bearing vector $\mathbf{f}$ and rotation cube $\mathcal{C}_r$, centred at angle-axis vector $\mathbf{r}_0$ with vertices $\{\mathbf{r}_i\}_{i\in[1,8]}$ and an edge parametrisation of $\mathbf{r}(\lambda) = \mathbf{r}_i + \lambda(\mathbf{r}_j - \mathbf{r}_i)$, is as follows.

(i) For each edge, evaluate the sign of the derivative of the angle function $\angle(\mathtt{R}^{-1}_{\mathbf{r}(\lambda)}\mathbf{f}, \mathtt{R}^{-1}_{\mathbf{r}_0}\mathbf{f})$ with respect to $\lambda$ at $\lambda = 0$ and $\lambda = 1$ using (12) and (13);
(ii) if (12) is positive and (13) is negative, use golden-section search [5] to find the angle maximiser on that edge, using a tolerance of $\pi/2048$, and add $\pi/2048$ to the result;
(iii) otherwise, the angle maximiser on that edge is a vertex: evaluate the angle with respect to the projected cube centre at both vertices and choose the maximum; and
(iv) choose the overall maximum angle as $\psi_r$.

Note that golden section search terminates at a tolerance of $\pi/2048$. By Lemma 1, the bound is therefore at most $\pi/2048 = 0.088°$ incorrect, a value that is added to the upper bound to ensure correctness.

We now provide the derivative of the rotation angle function in Lemma A.1. Given a unit 3D bearing vector $\mathbf{f}$ and a rotation cube $\mathcal{C}_r$ centred at $\mathbf{r}_0$ with vertices $\{\mathbf{r}_i\}_{i\in[1,8]}$, the rotation angle function with respect to $\lambda$, for an edge parametrisation of $\mathbf{r}(\lambda) = \mathbf{r}_i + \lambda(\mathbf{r}_j - \mathbf{r}_i)$ with $\lambda \in [0, 1]$, is

$$A(\lambda) = \arccos\left((\mathtt{R}^{-1}_{\mathbf{r}_0}\mathbf{f}) \cdot (\mathtt{R}^{-1}_{\mathbf{r}(\lambda)}\mathbf{f})\right). \tag{4}$$

**Lemma A.1.** *(Derivative of the rotation angle function) Given a unit 3D bearing vector* $\mathbf{f}$ *and a rotation cube* $\mathcal{C}_r$ *centred at* $\mathbf{r}_0$ *with vertices* $\{\mathbf{r}_i\}_{i\in[1,8]}$*, then*

$$\frac{dA}{d\lambda} = \frac{-\mathbf{f}^\intercal \mathtt{R}_{\mathbf{r}_0}\mathtt{R}^\intercal_{\mathbf{r}(\lambda)}[\mathbf{f}]_\times \left(\mathbf{r}(\lambda)\mathbf{r}(\lambda)^\intercal - (\mathtt{R}_{\mathbf{r}(\lambda)} - I)[\mathbf{r}(\lambda)]_\times\right)\left(\mathbf{r}_j - \mathbf{r}_i\right)}{\|\mathbf{r}(\lambda)\|^2\sqrt{1 - (\mathbf{f}^\intercal \mathtt{R}_{\mathbf{r}_0}\mathtt{R}^\intercal_{\mathbf{r}(\lambda)}\mathbf{f})^2}}. \tag{5}$$

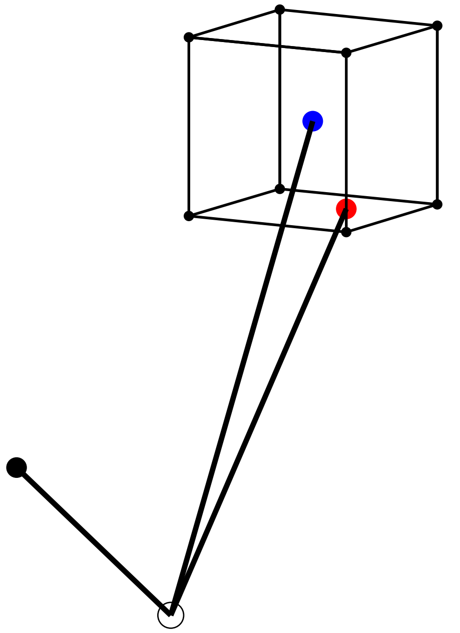

(a) Rotation cube in angle-axis space with centre $\mathbf{r}_0$ (blue dot), projected angle maximiser $\mathbf{r}^*$ (red dot), origin (black circle) and unrotated 3D point $\mathbf{p}$ (black dot). Cube edges and vertices are shown as thin black lines and small black dots respectively.

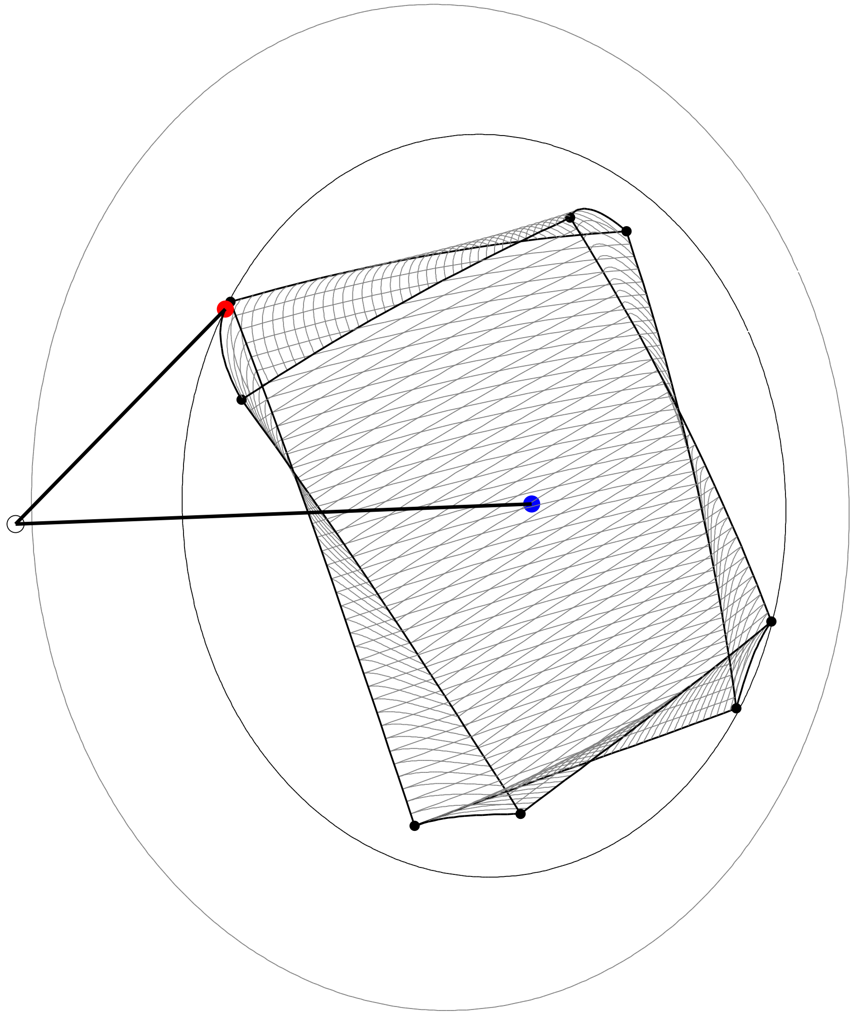

(b) Rotation of 3D point $\mathbf{p}$ by angle-axis vectors on the surface of the cube with centre-rotated point $\mathtt{R}_{\mathbf{r}_0}\mathbf{p}$ (blue dot), angle maximiser $\mathtt{R}_{\mathbf{r}^*}\mathbf{p}$ (red dot) and origin (black circle). 40 equally-spaced lines across each face are plotted in grey. All points and lines, other than the origin and lines to the origin, lie on the surface of a sphere with radius $\|\mathbf{p}\|$. Cube edges and vertices are shown as thin black lines and small black dots respectively. The weak rotation uncertainty angle $\psi_r^w$ corresponds to the aperture angle of the cone formed by the origin and the grey circle. Our rotation uncertainty angle $\psi_r$ corresponds to the aperture angle of the cone formed by the origin and the black circle.

Figure A.1. A random rotation cube and the rotation of a random 3D point by all angle-axis vectors on the surface of that cube. Observe that the rotation vector that maximises the angle $\angle(\mathtt{R}_{\mathbf{r}}\mathbf{p}, \mathtt{R}_{\mathbf{r}_0}\mathbf{p})$ lies on a cube edge. Also observe that rotation vectors on the face of the cube (grey lines in the projection) do not rotate the point beyond the convex hull of the point rotated by the edges. Best viewed in colour.

*Proof.* Equation (5) can be derived as follows:

$$\mathrm{d}A = \frac{-1}{\sqrt{1-(\mathbf{f}^\intercal \mathtt{R}_{\mathbf{r}_0}\mathtt{R}_{\mathbf{r}(\lambda)}^\intercal \mathbf{f})^2}} \mathrm{d}\big((\mathtt{R}_{\mathbf{r}_0}^{-1}\mathbf{f}) \cdot (\mathtt{R}_{\mathbf{r}(\lambda)}^{-1}\mathbf{f})\big) \tag{6}$$

$$= \frac{-1}{\sqrt{1-(\mathbf{f}^\intercal \mathtt{R}_{\mathbf{r}_0}\mathtt{R}_{\mathbf{r}(\lambda)}^\intercal \mathbf{f})^2}} \mathbf{f}^\intercal \mathtt{R}_{\mathbf{r}_0} \mathrm{d}\big(\mathtt{R}_{\mathbf{r}(\lambda)}^\intercal \mathbf{f}\big) \tag{7}$$

$$= \frac{-1}{\sqrt{1-(\mathbf{f}^\intercal \mathtt{R}_{\mathbf{r}_0}\mathtt{R}_{\mathbf{r}(\lambda)}^\intercal \mathbf{f})^2}} \mathbf{f}^\intercal \mathtt{R}_{\mathbf{r}_0} \mathrm{d}\big(\mathtt{R}_{-\mathbf{r}(\lambda)} \mathbf{f}\big) \tag{8}$$

$$= \frac{-1}{\sqrt{1-(\mathbf{f}^\intercal \mathtt{R}_{\mathbf{r}_0}\mathtt{R}_{\mathbf{r}(\lambda)}^\intercal \mathbf{f})^2}} \mathbf{f}^\intercal \mathtt{R}_{\mathbf{r}_0} \left( -\mathtt{R}_{-\mathbf{r}(\lambda)}[\mathbf{f}]_\times \frac{(-\mathbf{r}(\lambda))(-\mathbf{r}(\lambda))^\intercal + (\mathtt{R}_{-\mathbf{r}(\lambda)}^\intercal - I)[-\mathbf{r}(\lambda)]_\times}{\|-\mathbf{r}(\lambda)\|^2} \right) \mathrm{d}(-\mathbf{r}(\lambda)) \tag{9}$$

$$= \frac{-1}{\sqrt{1-(\mathbf{f}^\intercal \mathtt{R}_{\mathbf{r}_0}\mathtt{R}_{\mathbf{r}(\lambda)}^\intercal \mathbf{f})^2}} \mathbf{f}^\intercal \mathtt{R}_{\mathbf{r}_0} \left( -\mathtt{R}_{\mathbf{r}(\lambda)}^\intercal[\mathbf{f}]_\times \frac{\mathbf{r}(\lambda)\mathbf{r}(\lambda)^\intercal - (\mathtt{R}_{\mathbf{r}(\lambda)} - I)[\mathbf{r}(\lambda)]_\times}{\|\mathbf{r}(\lambda)\|^2} \right) \mathrm{d}(-\mathbf{r}(\lambda)) \tag{10}$$

$$= \frac{-1}{\sqrt{1-(\mathbf{f}^\intercal \mathtt{R}_{\mathbf{r}_0}\mathtt{R}_{\mathbf{r}(\lambda)}^\intercal \mathbf{f})^2}} \mathbf{f}^\intercal \mathtt{R}_{\mathbf{r}_0} \left( \mathtt{R}_{\mathbf{r}(\lambda)}^\intercal[\mathbf{f}]_\times \frac{\mathbf{r}(\lambda)\mathbf{r}(\lambda)^\intercal - (\mathtt{R}_{\mathbf{r}(\lambda)} - I)[\mathbf{r}(\lambda)]_\times}{\|\mathbf{r}(\lambda)\|^2} \right) (\mathbf{r}_j - \mathbf{r}_i)\mathrm{d}\lambda \tag{11}$$

where (9) uses Result 1 from [3] and the derivative follows from the differential. □

Since the derivative is computationally expensive to calculate, we only evaluate it at the vertices. In addition, we only require the sign of the result, which simplifies the equation. Corollary A.1 presents the relevant results.

**Corollary A.1.** *(Sign of the derivative of the rotation angle function at the vertices) Given a unit 3D bearing vector* $\mathbf{f}$ *and a rotation cube* $\mathcal{C}_r$ *centred at* $\mathbf{r}_0$ *with vertices* $\{\mathbf{r}_i\}_{i\in[1,8]}$*, then*

$$\operatorname{sgn} \frac{dA}{d\lambda}\bigg|_{\lambda=0} = \operatorname{sgn} -\mathbf{f}^\intercal \mathtt{R}_{\mathbf{r}_0} \mathtt{R}_{\mathbf{r}_i}^\intercal [\mathbf{f}]_\times \Big(\mathbf{r}_i \mathbf{r}_i^\intercal - (\mathtt{R}_{\mathbf{r}_i} - I)[\mathbf{r}_i]_\times\Big)\Big(\mathbf{r}_j - \mathbf{r}_i\Big) \tag{12}$$

*and*

$$\operatorname{sgn} \frac{dA}{d\lambda}\bigg|_{\lambda=1} = \operatorname{sgn} -\mathbf{f}^\intercal \mathtt{R}_{\mathbf{r}_0} \mathtt{R}_{\mathbf{r}_j}^\intercal [\mathbf{f}]_\times \Big(\mathbf{r}_j \mathbf{r}_j^\intercal - (\mathtt{R}_{\mathbf{r}_j} - I)[\mathbf{r}_j]_\times\Big)\Big(\mathbf{r}_j - \mathbf{r}_i\Big). \tag{13}$$

## B. Tighter Upper Bound: Implementation Details

The upper bound given in Theorem 3 requires the evaluation of $\Gamma(\mathbf{f}, \mathbf{p})$ for a given translation cuboid $\mathcal{C}_t$. If the ray through $\mathbf{f}$ passes through the cube $\mathbf{p}_\mathbf{t}^{\mathbf{r}_0}$ for $\mathbf{t} \in \mathcal{C}_t$, the angle $\angle(\mathbf{f}, \mathbf{p}_\mathbf{t}^{\mathbf{r}_0})$ is zero. Otherwise, $\angle(\mathbf{f}, \mathbf{p}_\mathbf{t}^{\mathbf{r}_0})$ is equal to the angle between the $\mathbf{f}$ and the point on the skeleton of the cube (vertices and edges) with least angular displacement from $\mathbf{f}$. Thus, for the translation domain $\mathcal{C}_t$ with skeleton $\mathcal{S}k_t$,

$$\Gamma(\mathbf{f}, \mathbf{p}) = \begin{cases} \max\limits_{\mathbf{t}\in\mathcal{S}k_t} \mathbf{1}\big(\theta - \angle(\mathbf{f}, \mathbf{p}_\mathbf{t}^{\mathbf{r}_0}) + \psi_r(\mathbf{f}, \mathcal{C}_r)\big) & \text{if } \angle(\mathbf{f}, \mathbf{p}_{\mathbf{t}_0}^{\mathbf{r}_0}) > \psi_t(\mathbf{p}, \mathcal{C}_t) \\ 1 & \text{else.} \end{cases} \tag{14}$$

The key here is finding $\angle(\mathbf{f}, \mathbf{p}_\mathbf{t}^{\mathbf{r}_0})$ which maximises $\Gamma$ over the skeleton. For the first case, the implementation needs to find $\mathbf{p}_\mathbf{t}^{\mathbf{r}_0}$ with least angular displacement from $\mathbf{f}$. We use the following technique:

(i) find octant of $\mathbf{p} - \mathbf{t}_0$ and project the cube to the unit sphere as a spherical hexagon;
(ii) determine in which lune of the spherical hexagon (induced by the spherical hexagon) $\mathtt{R}_{\mathbf{r}_0}$ resides; and
(iii) solve for point on hexagon edge in that lune with least angular displacement from $\mathtt{R}_{\mathbf{r}_0}$.

We know from the data structure design that all translated points $\mathbf{p} - \mathbf{t}$ for $\mathbf{t} \in \mathcal{C}_t$ lie entirely in one octant of $\mathbb{R}^3$. Finding the octant (i) enables us to project the cube to a spherical hexagon on the unit sphere. That is, we can determine the 6 vertices of the cube that form the vertices of the spherical hexagon after projection and the order in which they cycle. This has simplified the problem to one of finding the closest point on the spherical hexagon to the rotated bearing vector. Finding which lune the rotated bearing lies in (ii) further simplifies the problem to one of finding the closest point on a geodesic to the rotated bearing vector. This can be solved in closed form (iii).

## C. Precomputing Angles on the Sphere

The nested structure of this implementation may be exploited by pre-computing the angle between the translated 3D points and any location on the unit sphere. Thus, for a fixed translation, the angle between any rotated bearing vector and its rotationally-closest 3D point may be pre-computed. This is essentially the analogue of a distance transform on the surface of the sphere $S^2$, in that the sphere is discretised and a look-up table constructed. By using this precomputation, the $\max$ operation in (27) and (28) is reduced from $\mathcal{O}(M)$ to $\mathcal{O}(1)$.

The procedure for constructing this look-up table follows. We subdivide the sphere into 98304 regions by projecting it onto an enclosing cube whose faces are partitioned with quad-trees. The configuration chosen ensures that the maximum angle between an arbitrary point and its nearest cell centre is 0.6°. We use a linear projection onto the cube, which facilitates rapid conversion from a unit vector to a location in the data structure. The disadvantage of a linear projection is that the cell sizes are not uniform, although they all respect the angle condition given above.

Mathematically, the effect of using this data structure is to relax $\theta$ by up to 0.6°. This means that the result is no longer optimal with respect to $\theta$, although it should be near-optimal. We did not use this feature in the experiments, because it cannot ensure optimality, although it is useful for solving problems with large $M$, that is, many 3D points.

## D. Comparison with Weaker Bounds

The weaker sphere-based uncertainty angles $\psi_r^w$ and $\psi_t^w$ given in (7) and (16) appeared originally in [4] and [1] respectively. The tighter cuboid-based uncertainty angles $\psi_r$ and $\psi_t$ given in (10) and (13) are original to this work and lead to tighter bounds on the objective function. This can be seen from Theorems 1 and 2, where it is clear that $\bar{f} - \underline{f}$ is smaller when the uncertainty angles $\psi_r$ and $\psi_t$ are smaller. The proofs that $\psi_r \leqslant \psi_r^w$ and $\psi_t \leqslant \psi_t^w$ will now be given.

**Lemma D.1.** *(Rotation uncertainty angle inequality) Given a 3D bearing vector* $\mathbf{f}$ *and a rotation cube* $\mathcal{C}_r$ *of half-side length* $\delta_r$ *centred at* $\mathbf{r}_0$*, then*

$$\psi_r(\mathbf{f}, \mathcal{C}_r) \leqslant \psi_r^w(\mathcal{C}_r). \tag{15}$$

*Proof.* Inequality (15) can be derived as follows:

$$\begin{aligned}
\psi_r(\mathbf{f}, \mathcal{C}_r) &= \min\left\{\max_{\mathbf{r}\in\mathcal{S}_r} \angle(\mathtt{R}_\mathbf{r}\mathbf{f}, \mathtt{R}_{\mathbf{r}_0}\mathbf{f}), \pi\right\} && (16)\\
&= \min\left\{\angle(\mathtt{R}_{\mathbf{r}^*}\mathbf{f}, \mathtt{R}_{\mathbf{r}_0}\mathbf{f}), \pi\right\} && (17)\\
&\leqslant \min\left\{\sqrt{3}\delta_r, \pi\right\} && (18)\\
&= \psi_r^w(\mathcal{C}_r) && (19)
\end{aligned}$$

where (17) replaces the maximisation with the $\arg\max$ rotation $\mathbf{r}^*$ and (18) follows from Lemma 2. □

**Lemma D.2.** *(Translation uncertainty angle inequality) Given a 3D point* $\mathbf{p}$ *and a translation cuboid* $\mathcal{C}_t$ *of half-side length* $\delta_t$ *centred at* $\mathbf{t}_0$*, then*

$$\psi_t(\mathbf{p}, \mathcal{C}_t) \leqslant \psi_t^w(\mathbf{p}, \mathcal{C}_t). \tag{20}$$

*Proof.* Inequality (20) can be derived as follows. For $\|\mathbf{p} - \mathbf{t}_0\| \geqslant \rho_t$, which is guaranteed for $\rho_t \leqslant \zeta$,

$$\begin{aligned}
\psi_t(\mathbf{p}, \mathcal{C}_t) &= \max_{\mathbf{t}\in\mathcal{V}_t} \angle(\mathbf{p} - \mathbf{t}, \mathbf{p} - \mathbf{t}_0) && (21)\\
&\leqslant \max_{\mathbf{t}\in S_t^2} \angle(\mathbf{p} - \mathbf{t}, \mathbf{p} - \mathbf{t}_0) && (22)\\
&= \arcsin\left(\frac{\rho_t}{\|\mathbf{p} - \mathbf{t}_0\|}\right) && (23)\\
&= \psi_t^w(\mathbf{p}, \mathcal{C}_t) && (24)
\end{aligned}$$

where (22) follows from maximising the angle over the circumsphere $S_t^2$ of the cuboid instead of the vertices and (23) is shown in [1] with $\rho_t$ being the half space diagonal of the translation subcuboid $\mathcal{C}_t$. For $\|\mathbf{p} - \mathbf{t}_0\| < \rho_t$, $\psi_t \leqslant \pi = \psi_t^w$. □

Therefore, the weaker uncertainty angles $\psi_r^w$ and $\psi_t^w$ are larger than the uncertainty angles $\psi_r$ and $\psi_t$ for a given rotation or translation subcuboid. Consequently, the bounds using $\psi_r$ and $\psi_t$ are tighter than those using $\psi_r^w$ and $\psi_t^w$.

## E. Proof of Algorithm Convergence

A requirement of branch-and-bound is that the upper and lower bounds converge as the size of the branch tends to zero. The convergence of the bounds can be proved as follows. It is clear that the upper bound (19) is equal to the lower bound (17) when the uncertainty angles $\psi_r(\mathbf{f}, \mathcal{C}_r)$ and $\psi_t(\mathbf{p}, \mathcal{C}_t)$ are zero. Similarly, the tighter upper bound (22) is equal to the lower bound when the rotation uncertainty angle $\psi_r(\mathbf{f}, \mathcal{C}_r)$ is zero and the translation subcuboid $\mathcal{C}_t$ is of size zero, since then $\angle(\mathbf{f}, \mathbf{p}_\mathbf{t}^{\mathbf{r}_0}) = \angle(\mathbf{f}, \mathbf{p}_{\mathbf{t}_0}^{\mathbf{r}_0})$ for $\mathbf{t} \in \mathcal{C}_t$. It remains to be seen that $\psi_r(\mathbf{f}, \mathcal{C}_r)$ and $\psi_t(\mathbf{p}, \mathcal{C}_t)$ tend to zero as the size of the subcuboids $\mathcal{C}_r$ and $\mathcal{C}_t$ tend to zero, irrespective of the value of $\mathbf{f}$ or $\mathbf{p}$.

The rotation uncertainty angle $\psi_r(\mathbf{f}, \mathcal{C}_r)$ involves a maximisation over all rotations on the surface of the subcube $\mathcal{C}_r$. As the subcube size tends to zero, in the limit the surface and centre of the cube become identified and therefore the angle $\angle(\mathtt{R}_\mathbf{r}\mathbf{f}, \mathtt{R}_{\mathbf{r}_0}\mathbf{f})$ equals zero. The translation uncertainty angle $\psi_t(\mathbf{p}, \mathcal{C}_t)$ involves a maximisation over all translations on the vertices of the subcuboid $\mathcal{C}_t$. As the subcuboid size tends to zero, in the limit the vertices and centre of the cuboid become identified and therefore the angle $\angle(\mathbf{p} - \mathbf{t}, \mathbf{p} - \mathbf{t}_0)$ equals zero. The point $\mathbf{p}$ cannot lie inside the subcuboid for a sufficiently small cuboid, since the translation domain has been restricted to exclude translations for which $\|\mathbf{p} - \mathbf{t}\| < \zeta$. Therefore the upper and lower bounds converge as the size of subcuboids (branches) tend to zero.

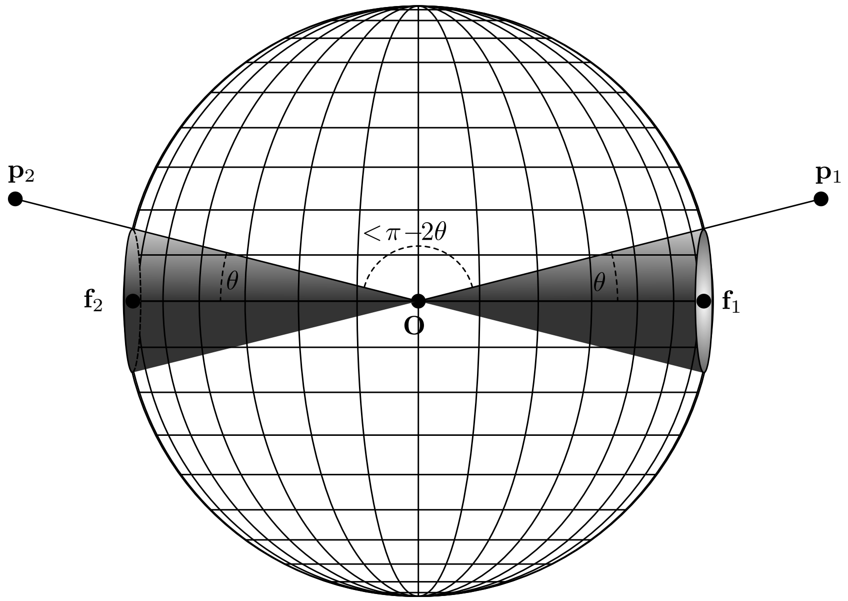


Figure E.1. Example of a critical configuration (rotation-only). The angle between the 3D point vectors $\angle(\mathbf{p}_1, \mathbf{p}_2)$ is infinitesimally less than $\pi - 2\theta$. To prove that the maximum number of inliers is 1, infinitesimally small rotation subcubes will be required.

However, an advantage of the inlier maximisation formulation is that the gap between the bounds becomes exactly zero well before the branch size becomes infinitesimal. There are nonetheless critical configurations of points and bearing vectors for which the bounds will only converge in the limit. The simplest case is illustrated in Figure E.1. In this rotation-only example, the angle between the 3D point vectors is infinitesimally less than $\pi - 2\theta$. To prove that the maximum number of inliers is 1, infinitesimally small rotation subcubes will be required.

In order to guarantee that the algorithm terminates in finite time, a small tolerance value $\eta$ must be subtracted from the uncertainty angles. That is, replace the uncertainty angles in all the formulae with their primed versions: $\psi_r' = \psi_r - \eta$ and $\psi_t' = \psi_t - \eta$. For the tighter upper bound, $\eta$ also has to be added to $\angle(\mathbf{f}, \mathbf{p}_{\mathbf{t}}^{\mathbf{r}_0})$. Writing the nested bounds with the uncertainty angle tolerances gives the following. The upper bound $\bar{\nu} \triangleq \bar{\nu}_t$ (19) for the translation cuboid $\mathcal{C}_t$ is found by running rotation BB until convergence with the following bounds

$$\underline{\nu}_r \triangleq \sum_{\mathbf{f}\in\mathcal{F}} \max_{\mathbf{p}\in\mathcal{P}} \mathbf{1}\big(\theta - \angle(\mathbf{f}, \mathbf{p}_{\mathbf{t}_0}^{\mathbf{r}_0}) + \psi_t'(\mathbf{p})\big) \tag{25}$$

$$\bar{\nu}_r \triangleq \sum_{\mathbf{f}\in\mathcal{F}} \max_{\mathbf{p}\in\mathcal{P}} \mathbf{1}\big(\theta - \angle(\mathbf{f}, \mathbf{p}_{\mathbf{t}_0}^{\mathbf{r}_0}) + \psi_t'(\mathbf{p}) + \psi_r'(\mathbf{f})\big). \tag{26}$$

The tighter upper bound (22) instead uses

$$\underline{\nu}_r \triangleq \sum_{\mathbf{f}\in\mathcal{F}} \max_{\mathbf{p}\in\mathcal{P}, \mathbf{t}\in\mathcal{C}_t} \mathbf{1}\big(\theta - \angle(\mathbf{f}, \mathbf{p}_{\mathbf{t}}^{\mathbf{r}_0}) - \eta\big) \tag{27}$$

$$\bar{\nu}_r \triangleq \sum_{\mathbf{f}\in\mathcal{F}} \max_{\mathbf{p}\in\mathcal{P}, \mathbf{t}\in\mathcal{C}_t} \mathbf{1}\big(\theta - \angle(\mathbf{f}, \mathbf{p}_{\mathbf{t}}^{\mathbf{r}_0}) - \eta + \psi_r'(\mathbf{f})\big). \tag{28}$$

The lower bound $\underline{\nu} \triangleq \underline{\nu}_t$ (17) for $\mathcal{C}_t$ is found by running rotation BB until convergence using bounds (25) and (26) with $\psi_t'$ set to zero. That is, the bounds

$$\underline{\nu}_r \triangleq \sum_{\mathbf{f}\in\mathcal{F}} \max_{\mathbf{p}\in\mathcal{P}} \mathbf{1}\big(\theta - \angle(\mathbf{f}, \mathbf{p}_{\mathbf{t}_0}^{\mathbf{r}_0})\big) \tag{29}$$

$$\bar{\nu}_r \triangleq \sum_{\mathbf{f}\in\mathcal{F}} \max_{\mathbf{p}\in\mathcal{P}} \mathbf{1}\big(\theta - \angle(\mathbf{f}, \mathbf{p}_{\mathbf{t}_0}^{\mathbf{r}_0}) + \psi_r'(\mathbf{f})\big). \tag{30}$$

In this work, $\eta$ was set to machine epsilon for maximal precision. In C++, this can be accessed by using the command `std::numeric_limits<float>::epsilon()`.

## F. Time Complexity

Explicitly including the tolerance $\eta$ in the bound formulae makes it possible to derive a bound on the worst-case search tree depth and thereby obtain the time complexity of the algorithm. In terms of the size of the input, the GOPAC algorithm is $O(MN)$, or $O(N)$ if angle precomputation is used, where $M$ is the number of 3D points and $N$ is the number of bearing vectors. However, the notation conceals a very large constant. Including the constant factors that can be selected by the user yields $O(\rho_{t_0}^3 \zeta^{-3} \eta^{-6} MN)$, where $\rho_{t_0}$ is the half space diagonal of the initial translation cuboids, that is one-quarter the space diagonal of the translation domain, and $\zeta$ and $\eta$ are small previously-defined constants set by the user.

Calculating the upper and lower bounds involves a summation over $\mathcal{F}$ and a maximisation over $\mathcal{P}$, therefore the complexity is $O(MN)$. If angle precomputation is used, the maximisation becomes a constant-time lookup leading to a bound complexity of $O(N)$. However, it is as of yet unclear how the number of iterations (explored subcuboids) depends on the inputs. The central finding is that branch-and-bound is exponential in the worst-case tree search depth $D$, but $D$ is logarithmic in $\eta^{-1}$. Therefore the complexity of BB is polynomial in $\eta^{-1}$, where $\eta$ is the angle tolerance. Rotation and translation search will be treated separately before being combined into an analysis of nested rotation and translation search.

**Theorem 1.** *(Rotation Search Depth and Complexity) Let $\rho_{r_0} = \sqrt{3}\delta_{r_0} = \sqrt{3}\pi/2$ be the half space diagonal of the initial rotation subcube $\mathcal{C}_{r_0}$. Then*

$$D_r = \max\left\{\left\lceil \log_2 \frac{\rho_{r_0}}{\eta} \right\rceil, 0\right\} \tag{31}$$

*is an upper bound on the worst-case rotation tree search depth for an uncertainty angle tolerance $\eta$ and $O(\eta^{-3})$ is the time complexity of rotation BB search.*

*Proof.* Rotation BB converges when $\underline{\nu}_r \geqslant \bar{\nu}_r$. For any $\psi_t'(\mathbf{p}, \mathcal{C}_t)$ in (25) and (26), $\underline{\nu}_r \geqslant \bar{\nu}_r$ when $\psi_r'(\mathbf{f}, \mathcal{C}_r) \leqslant 0$ or equivalently $\psi_r(\mathbf{f}, \mathcal{C}_r) \leqslant \eta$ for all $\mathbf{f} \in \mathcal{F}$. Now,

$$\begin{aligned}
\psi_r(\mathbf{f}, \mathcal{C}_r) &= \min\left\{\max_{\mathbf{r}\in\mathcal{S}_r} \angle(\mathtt{R}_\mathbf{r}\mathbf{f}, \mathtt{R}_{\mathbf{r}_0}\mathbf{f}), \pi\right\} && (32)\\
&= \min\left\{\angle(\mathtt{R}_{\mathbf{r}^*}\mathbf{f}, \mathtt{R}_{\mathbf{r}_0}\mathbf{f}), \pi\right\} && (33)\\
&\leqslant \min\left\{\sqrt{3}\delta_r, \pi\right\} && (34)\\
&\leqslant \rho_r && (35)
\end{aligned}$$

where (33) replaces the maximisation with the $\arg\max$ rotation $\mathbf{r}^*$, (34) follows from Lemma 2 and $\rho_r$ is the half space diagonal of the rotation subcube $\mathcal{C}_r$. At rotation search tree depth $D_r$, the half space diagonal is given by

$$\rho_{r_{D_r}} = \frac{1}{2}\rho_{r_{D_r - 1}} = \frac{1}{2^{D_r}}\rho_{r_0}. \tag{36}$$

Substituting into (35) gives

$$\psi_r(\mathbf{f}, \mathcal{C}_{r_{D_r}}) \leqslant \rho_{r_{D_r}} = 2^{-D_r}\rho_{r_0}. \tag{37}$$

To find the worst-case rotation search tree depth, the constraint $\psi_r(\mathbf{f}, \mathcal{C}_r) \leqslant \eta$ is applied:

$$\psi_r(\mathbf{f}, \mathcal{C}_{r_{D_r}}) \leqslant 2^{-D_r}\rho_{r_0} \leqslant \eta. \tag{38}$$

Taking the logarithm of both sides yields

$$D_r \geqslant \log_2 \frac{\rho_{r_0}}{\eta}. \tag{39}$$

Equation (31) follows from the requirement that $D_r$ be a non-negative integer. Now, rotation BB will have examined at most

$$N_r = 8(1 + 8 + 8^2 + \cdots + 8^{D_r}) = 8\frac{8^{D_r+1} - 1}{8 - 1} = \frac{8}{7}\left((2^{D_r+1})^3 - 1\right) \tag{40}$$

subcubes at search depth $D_r$, due to the octree structure. Finally, substituting (31) into (40) and simplifying using Bachmann–Landau notation gives

$$N_r = O\left(\left(\frac{\rho_{r_0}}{\eta}\right)^3\right) = O\left(\eta^{-3}\right). \tag{41}$$

The $\rho_{r_0}$ term is removed because it is a constant (equal to $\sqrt{3}\pi/2$) that is not selected by the user. □

The analysis of the worst-case search depth and time complexity for translation search proceeds in a similar manner.

**Theorem 2.** *(Translation Search Depth and Complexity) Let $\rho_{t_0}$ be the half space diagonal of the initial translation subcuboid $\mathcal{C}_{t_0}$. Then*

$$D_t = \max\left\{\left\lceil \log_2 \frac{\rho_{t_0}}{\zeta \sin\eta} \right\rceil, 0\right\} \tag{42}$$

*is an upper bound on the worst-case translation tree search depth for an uncertainty angle tolerance $\eta$ and $O(\rho_{t_0}^3 \zeta^{-3} \eta^{-3})$ is the time complexity of translation BB search.*

*Proof.* Translation BB converges when $\underline{\nu}_t \geqslant \bar{\nu}_t$. This condition is met when $\psi_t'(\mathbf{p}, \mathcal{C}_t) \leqslant 0$ or equivalently $\psi_t(\mathbf{p}, \mathcal{C}_t) \leqslant \eta$ for all $\mathbf{p} \in \mathcal{P}$. This can be seen by inspecting (25) and (29) and noting that at convergence the upper and lower rotation bounds will be equal. Now for $\|\mathbf{p} - \mathbf{t}_0\| \geqslant \rho_t$, which is guaranteed for $\rho_t \leqslant \zeta$,

$$\psi_t(\mathbf{p}, \mathcal{C}_t) = \max_{\mathbf{t} \in \mathcal{V}_t} \angle(\mathbf{p} - \mathbf{t}, \mathbf{p} - \mathbf{t}_0) \tag{43}$$

$$\leqslant \max_{\mathbf{t} \in S_t^2} \angle(\mathbf{p} - \mathbf{t}, \mathbf{p} - \mathbf{t}_0) \tag{44}$$

$$= \arcsin\left(\frac{\rho_t}{\|\mathbf{p} - \mathbf{t}_0\|}\right) \tag{45}$$

$$\leqslant \arcsin\left(\frac{\rho_t}{\zeta}\right) \tag{46}$$

where (44) follows from maximising the angle over the circumsphere $S_t^2$ of the cuboid instead of the vertices, (45) is shown in [1] with $\rho_t$ being the half space diagonal of the translation subcuboid $\mathcal{C}_t$, and (46) follows from the restriction of the translation domain such that $\|\mathbf{p} - \mathbf{t}\| \geqslant \zeta$. At translation search tree depth $D_t$, the half space diagonal of $\mathcal{C}_{t_{D_t}}$ is given by

$$\rho_{t_{D_t}} = \frac{1}{2}\rho_{t_{D_t - 1}} = \frac{1}{2^{D_t}}\rho_{t_0}. \tag{47}$$

Substituting into (46) gives

$$\psi_t(\mathbf{p}, \mathcal{C}_{t_{D_t}}) \leqslant \arcsin\left(\frac{\rho_{t_{D_t}}}{\zeta}\right) = \arcsin\left(\frac{\rho_{t_0}}{\zeta 2^{D_t}}\right). \tag{48}$$

To find the worst-case translation search tree depth, the constraint $\psi_t(\mathbf{p}, \mathcal{C}_t) \leqslant \eta$ is applied, resulting in

$$\psi_t(\mathbf{p}, \mathcal{C}_{t_{D_t}}) \leqslant \arcsin\left(\frac{\rho_{t_0}}{\zeta 2^{D_t}}\right) \leqslant \eta. \tag{49}$$

Taking the sine and logarithm of both sides yields

$$D_t \geqslant \log_2 \frac{\rho_{t_0}}{\zeta \sin\eta}. \tag{50}$$

Equation (42) follows from the requirement that $D_t$ be a non-negative integer. Now, translation BB will have examined at most

$$N_t = 8(1 + 8 + 8^2 + \cdots + 8^{D_t}) = 8\frac{8^{D_t+1} - 1}{8 - 1} = \frac{8}{7}\left((2^{D_t+1})^3 - 1\right) \tag{51}$$

subcuboids at search depth $D_t$. Finally, substituting (42) into (51) and simplifying using Bachmann–Landau notation and the Taylor expansion of $\sin\eta$ gives

$$N_t = O\left(\rho_{t_0}^3 \zeta^{-3} (\sin\eta)^{-3}\right) = O\left(\rho_{t_0}^3 \zeta^{-3} \eta^{-3}\right). \tag{52}$$

□

In the nested BB search structure detailed at the beginning of Section 5, for every translation subcuboid examined, rotation BB search is run once to find the lower translation bound and again to find the upper translation bound. Thus the number of rotation subcubes examined is at worst equal to $2N_tN_r$. For each rotation subcube, both the upper and lower bounds must be calculated, each with a time complexity of $O(MN)$. Thus the total number of bound calculations is at worst equal to $4N_tN_r$. Combining the time complexity analyses (41) and (52) with the time complexity of the bound calculations leads to the following corollary.

**Corollary F.1.** *(Time Complexity of GOPAC) Let $\rho_{t_0}$ be the half space diagonal of the initial translation subcuboid $\mathcal{C}_{t_0}$, $\zeta$ be the translation restriction parameter, $\eta$ be the uncertainty angle tolerance, $M$ be the number of 3D points and $N$ be the number of bearing vectors, then the time complexity of the GOPAC algorithm is given by*

$$O\left(\rho_{t_0}^3 \zeta^{-3} \eta^{-6} MN\right). \tag{53}$$

It is important to observe that experimental evaluation of runtime is more revealing for BB algorithms than time complexity analysis. The main reason to use BB is that it can prune large regions of the search space, reducing the size of the problem. This is not reflected in the complexity analysis.

# G. Additional Experiments and Results

## G.1. Synthetic Data Experiments: Cube Prior

In the paper, we applied a torus prior in order to be as fair to the local optimisation approaches as possible. However, in general, restrictive constraints on the rotation and translation cannot be easily obtained. A more realistic prior, that can still be used by BlindPnP [7] and SoftPOSIT [2] in order to facilitate comparison, is a cube prior. This constrains the camera centre to a cube with no restriction on rotation. The intent of this prior is to simulate the task of camera pose estimation with respect to a scene, such as locating a camera inside a building, instead of the torus prior which simulates the task of camera pose estimation with respect to an object, such as a teapot on a table.

We use a cube centred at a random location in $[-1, 1]^3$ with side-length 0.5m. Again, we use the Monte Carlo simulation framework of [7] for the experiments: $M$ random 3D points were generated from $[-1, 1]^3$; a fraction $\omega_{\text{3D}}$ of the 3D points were randomly selected as outliers to model occlusion; the inliers were projected to a virtual image $640 \times 480$ with an effective focal length of 800 and centre of $(320, 240)$ and normal noise was added with $\sigma = 2$ pixels; and random points were added to the image such that a fraction $\omega_{\text{2D}}$ of the 2D points were outliers.

BlindPnP represents this pose prior with a 50 component Gaussian mixture model, the means of which are used to initialise SoftPOSIT, as in [7]. We have increased the number of components from the 20 recommended by the authors to help model the increased rotation uncertainty. The mixture model was trained from a set of 200 random camera centres in the cube and a set of 200 uniform random rotation matrices, generated using the method in [6].

The results are shown in Figure G.1. Two success rates are reported: the fraction of trials where the true maximum number of inliers was found and the fraction where the correct pose was found, where the angle between the output rotation and the ground truth rotation is less than 0.1 radians and the camera centre error $\|\mathbf{t} - \mathbf{t}_{\text{GT}}\| / \|\mathbf{t}_{\text{GT}}\|$ relative to the ground truth $\mathbf{t}_{\text{GT}}$ is less than 0.1, as in [7]. The 2D and 3D outlier fractions were fixed to 0 when not being varied and multithreading was used in the 2D outlier experiments. Our method (GOPAC) outperforms the other methods by a significant margin. In particular, SoftPOSIT was unable to find the correct pose in all experiments, largely due to being unable to handle 3D points behind the camera. BlindPnP is also sensitive to 3D outliers behind the camera and is relatively slow with 50 mixture model components, as is reflected in its results. However, it was necessary to use 50 in order to obtain reasonable results for the camera pose. Moreover, without a strong rotation prior, both local methods have difficulty finding the best pose.

## G.2. Synthetic Data Experiments: Early Termination

The early termination strategy, referred to in the paper as "truncated GOPAC" or $\lfloor$GP$\rfloor$, is investigated further in this section. Recall that since the majority of the runtime of the algorithm is spent decreasing the upper bound, an early termination strategy will often attain the global optimum, although it will not be able to guarantee optimality. We repeated the 2D outlier experiments for the torus prior with random points to show the performance of our algorithm when it is terminated after 30s. At termination, the algorithm returns the best-so-far cardinality and camera pose, as well as a flag to indicate that the result is not guaranteed to be optimal. The results are shown in Figure G.2. It is clear that the method still performs very well even when terminated early, albeit without an optimality guarantee. For some applications, it may be worth sacrificing optimality for the significant decrease in runtime. For comparison, we also plot the results from the paper without truncation.

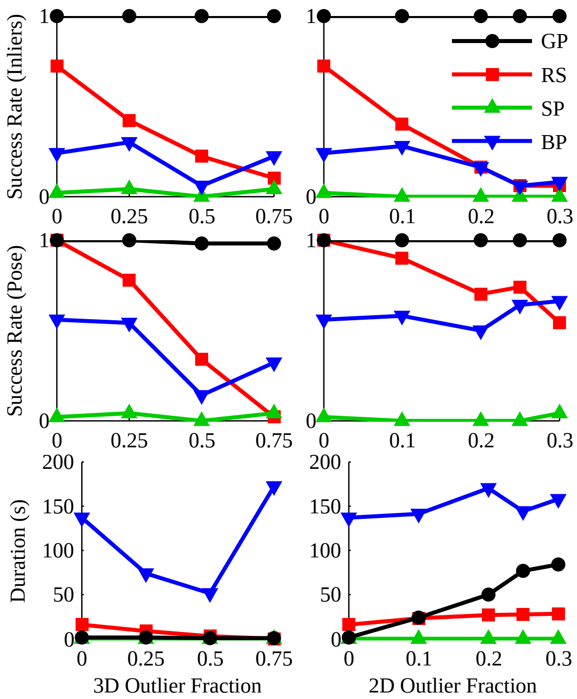


Figure G.1. Cube Prior. Mean success rates and median runtimes with respect to the 3D and 2D outlier fractions for the random points dataset, for 50 Monte Carlo simulations per parameter value with the cube prior. The 2D outlier fraction was fixed at 0 for the 3D outlier experiments and the 3D outlier fraction was fixed at 0 for the 2D outlier experiments.

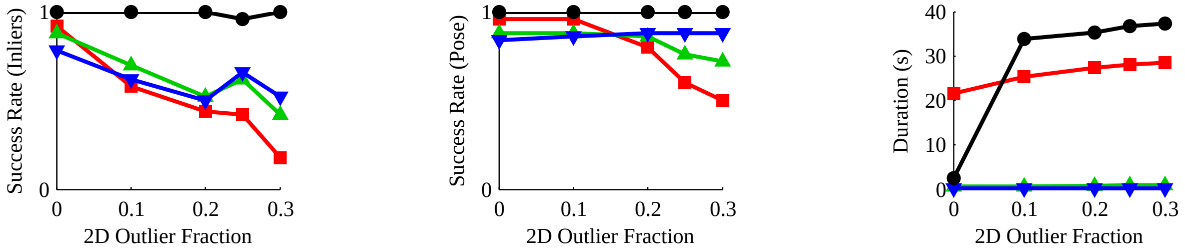


(a) Truncated GOPAC

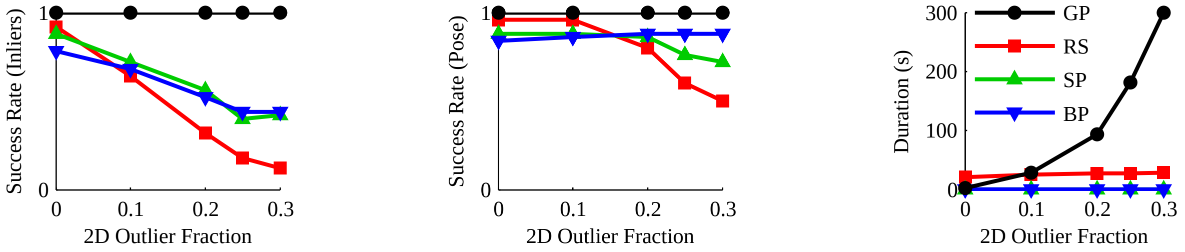


(b) Standard GOPAC

Figure G.2. A comparison of "truncated GOPAC" and standard GOPAC. Mean success rates and median runtimes with respect to the 2D outlier fractions for the random points dataset, for 50 Monte Carlo simulations per parameter value with the torus prior. The 3D outlier fraction was fixed at 0.

## G.3. Real Data Experiments

In this section, we present quantitative and qualitative results for a new dataset and additional quantitative and qualitative results for the experiments reported in Section 6.2. The new dataset was generated from a different scene ("Scene5") of the outdoor DATA61/2D3D dataset, using the same method described in Section 6.2. It consists of a 3D point-set with 98 points, a set of 11 images containing 30 2D features and a set of ground truth camera poses. In contrast to the residential scene reported in the main paper ("Scene1"), this scene is mixed-use, with residential and commercial or industrial areas, is less

Table G.1. Camera pose results for the supplementary DATA61/2D3D dataset ("Scene5"). Quartiles for translation error, rotation error and runtime and the mean inlier recall and success rates are reported. $\lfloor$GP$\rfloor$ denotes truncated GOPAC, where search is terminated after 30s, with no optimality guarantee. $\text{RS}_K$ denotes RANSAC with $K$ million iterations.

| Method | GP | $\lfloor$GP$\rfloor$ | $\text{RS}_{20}$ | $\text{RS}_{240}$ |
|---|---|---|---|---|
| Translation Error (m) | **1.59 / 2.03 / 11.2** | 1.70 / 2.72 / 11.3 | 7.79 / 31.5 / 45.8 | 1.74 / 4.11 / 14.9 |
| Rotation Error (°) | **2.14 / 3.28 / 179** | 1.95 / 3.70 / 179 | 117 / 179 / 179 | 3.52 / 140 / 179 |
| Recall (Inliers) | **1.00** | 0.98 | 0.78 | 0.86 |
| Success Rate (Inliers) | **1.00** | 0.55 | 0.00 | 0.09 |
| Success Rate (Pose) | **0.55** | **0.55** | 0.18 | 0.45 |
| Runtime (s) | 229 / 346 / 409 | 33 / 33 / 33 | 29 / 29 / 32 | 339 / 347 / 382 |

Table G.2. Camera pose results for the DATA61/2D3D dataset ("Scene1"). Quartiles for translation error, rotation error and runtime and the mean inlier recall and success rates are reported. $\lfloor$GP$\rfloor$ denotes truncated GOPAC, where search is terminated after 30s, with no optimality guarantee. $\text{RS}_K$ denotes RANSAC with $K$ million iterations.

| Method | GP | $\lfloor$GP$\rfloor$ | $\text{RS}_{20}$ | $\text{RS}_{280}$ |
|---|---|---|---|---|
| Translation Error (m) | **1.77 / 2.30 / 4.37** | 1.85 / 3.10 / 6.31 | 13.0 / 20.3 / 24.8 | 19.2 / 28.5 / 38.4 |
| Rotation Error (°) | **1.75 / 2.08 / 3.15** | 1.92 / 3.04 / 137 | 90.2 / 178 / 179 | 117 / 179 / 179 |
| Recall (Inliers) | **1.00** | 0.97 | 0.75 | 0.81 |
| Success Rate (Inliers) | **1.00** | 0.45 | 0.00 | 0.00 |
| Success Rate (Pose) | **0.82** | 0.64 | 0.09 | 0.09 |
| Runtime (s) | 311 / 477 / 496 | 33 / 34 / 34 | 33 / 34 / 35 | 453 / 471 / 480 |

spread out, and contains fewer buildings. For this experiment, we used an inlier threshold of $\theta = 2°$, multithreading and a 2D outlier fraction guess of $\omega_{2\text{D}} = 0.25$. The translation domain was $50 \times 5 \times 5$m, covering two lanes of the road, making use of the knowledge that the camera was mounted on a survey vehicle.

Qualitative results for the GOPAC and RANSAC algorithms are shown in Figure G.3 and quantitative results in Table G.1. GOPAC finds the optimal number of inliers for all frames and the correct camera pose for the majority of frames, despite the naïvety of the 2D/3D point extraction process. It is clear however that finding the optimal inlier set does not always correspond to finding the optimal pose for such a weak feature extraction procedure. In contrast, RANSAC performed better on this dataset than the original one, since it contains fewer, denser 3D clusters. This is beneficial for RANSAC because it reduces the implicitly-searched pose space, whereas it is disadvantageous for GOPAC because it does not reduce the search space and can mean that the inlier set at the correct pose has a lower cardinality than the inlier set at some incorrect poses. The main failure modes for GOPAC and RANSAC were 180° rotation flips, due to ambiguities arising from the low angular separation of points in the vertical direction.

Due to space restrictions, some additional quantitative and qualitative results for the experiments reported in Section 6.2 were not presented in the main paper. In Table G.2, Table 1 has been rewritten with quartile information for a more complete representation of the data. In Figure G.4, Figure 1 has been re-plotted at a larger scale. In Figures G.5, G.6 and G.7, we plot the remaining 10 images with the results obtained by GOPAC and RANSAC. It can be seen that there are two failure cases, with respect to camera pose (both remain optimal with respect to the number of inliers). In both cases, some of the extracted 2D features lie on non-building pixels, due to an error in the segmentation, which can be thought of as particularly undesirable 2D outliers. This is likely to have contributed to the algorithm finding the incorrect pose.

## References


[1] M. Brown, D. Windridge, and J.-Y. Guillemaut. Globally optimal 2D-3D registration from points or lines without correspondences. In *Proc. 2015 Int. Conf. Comput. Vision*, pages 2111–2119, 2015. 4, 7

[2] P. David, D. Dementhon, R. Duraiswami, and H. Samet. SoftPOSIT: simultaneous pose and correspondence determination. *Int. J. Comput. Vision*, 59(3):259–284, 2004. 8

[3] G. Gallego and A. Yezzi. A compact formula for the derivative of a 3-D rotation in exponential coordinates. *J. Mathematical Imaging Vision*, 51(3):378–384, 2015. 3

[4] R. I. Hartley and F. Kahl. Global optimization through rotation space search. *Int. J. Comput. Vision*, 82(1):64–79, 2009. 4

[5] J. Kiefer. Sequential minimax search for a maximum. *Proc. Am. Math. Soc.*, 4(3):502–506, 1953. 1

[6] F. Mezzadri. How to generate random matrices from the classical compact groups. *Notices Amer. Math. Soc.*, 54(5):592–604, 2007. 8

[7] F. Moreno-Noguer, V. Lepetit, and P. Fua. Pose priors for simultaneously solving alignment and correspondence. In *Proc. 2008 European Conf. Comput. Vision*, pages 405–418. Springer, 2008. 8

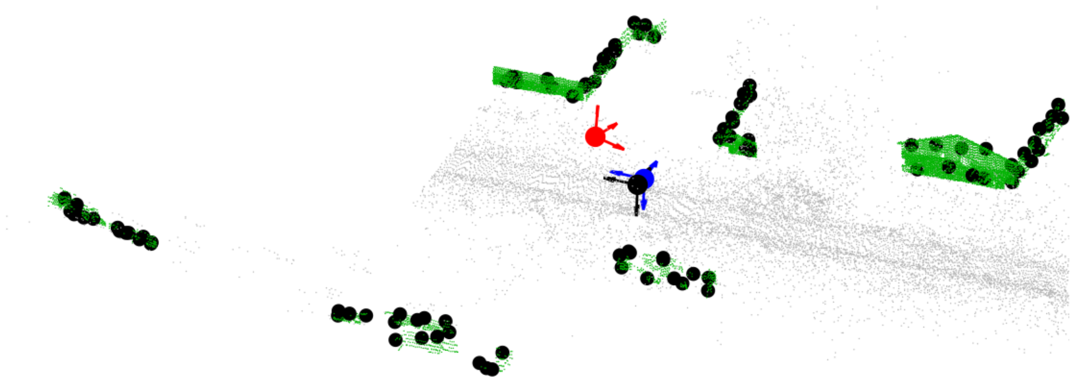

(a) 3D point-set (grey and green), 3D features (black dots) and ground-truth (black), RANSAC (red) and our (blue) camera poses. The ground-truth and our camera poses coincide, whereas the RANSAC pose has a translation offset and a 180° rotation offset. Best viewed in colour.

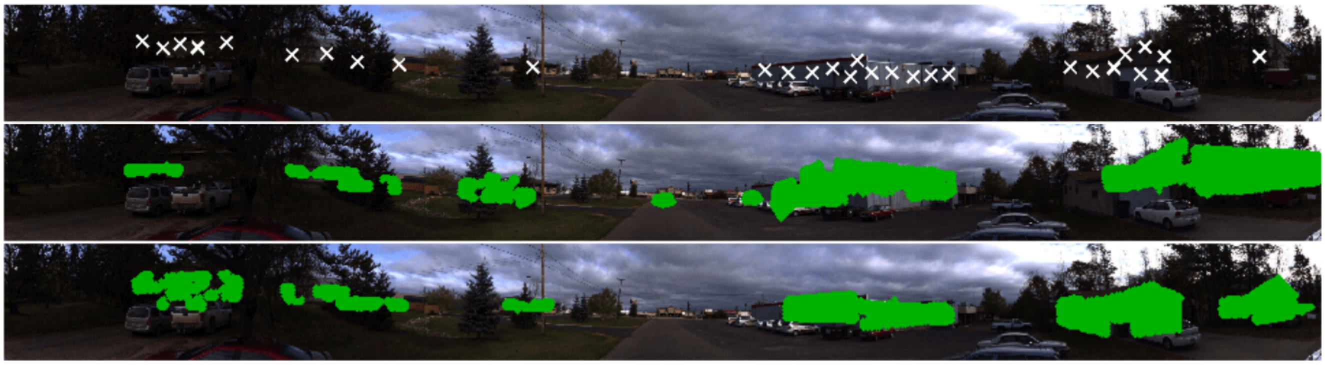

(b) Panoramic photograph and extracted 2D features (top), building points projected onto the image using the RANSAC camera pose (middle) and building points projected using our camera pose (bottom).

Figure G.3. Qualitative camera pose results for the supplementary DATA61/2D3D dataset (“Scene5”). The pose of the camera when it captured image 6 is shown, as is the projection of the building points onto image 6.

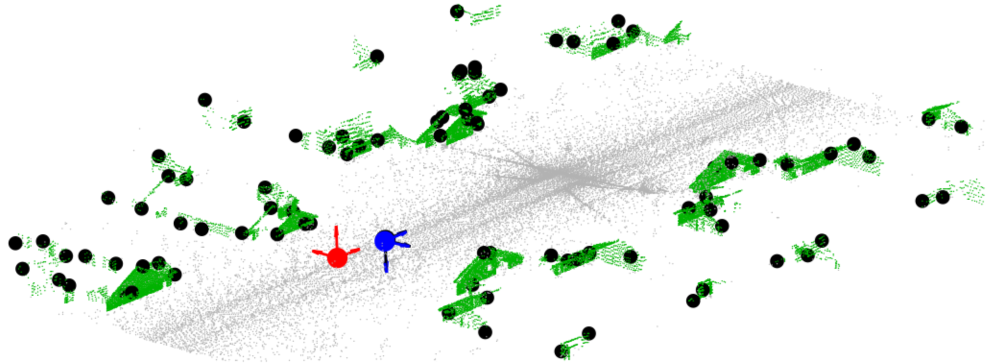

(a) 3D point-set (grey and green), 3D features (black dots) and ground-truth (black), RANSAC (red) and our (blue) camera poses. The ground-truth and our camera poses coincide, whereas the RANSAC pose has a translation offset and a $180°$ rotation offset. Best viewed in colour.

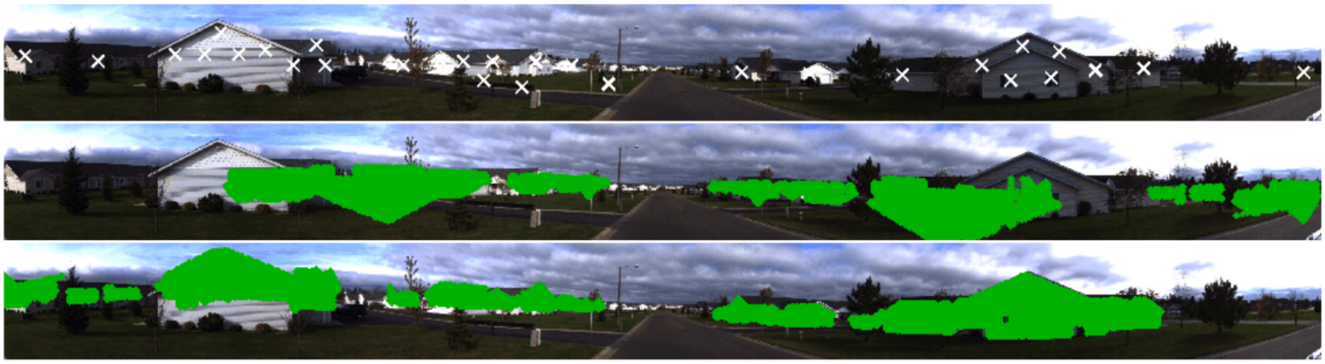

(b) Image 10. Panoramic photograph and extracted 2D features (top), building points projected onto the image using the RANSAC camera pose (middle) and building points projected using our camera pose (bottom).

Figure G.4. Estimating the pose of a calibrated camera from a single image within a large-scale, unorganised 3D point-set captured by vehicle-mounted laser scanner. Our method solves the absolute pose problem while simultaneously finding feature correspondences, using a globally-optimal branch-and-bound approach with tight novel bounds on the cardinality of the inlier set.

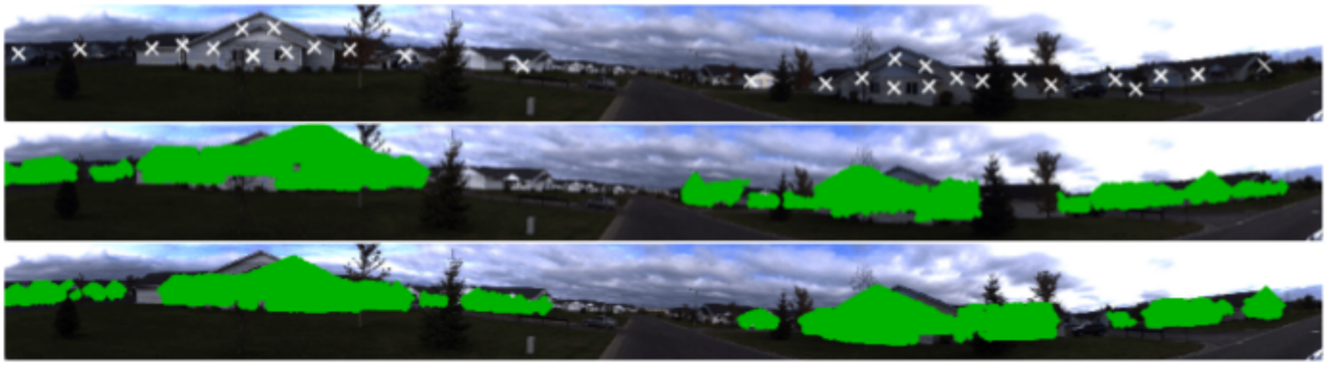

(a) Image 1: 2D features (top), building points projected using RANSAC camera pose (middle) and building points projected using our pose (bottom).

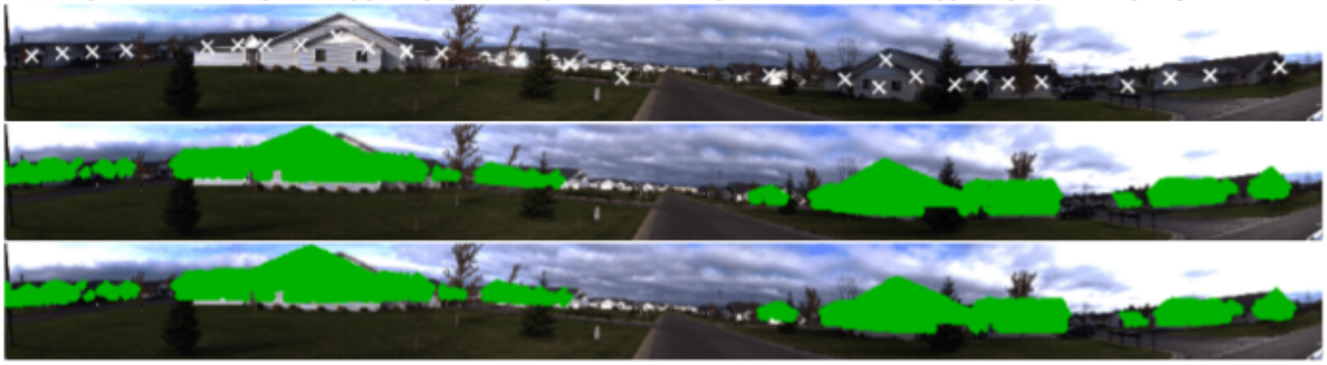

(b) Image 2: 2D features (top), building points projected using RANSAC camera pose (middle) and building points projected using our pose (bottom).

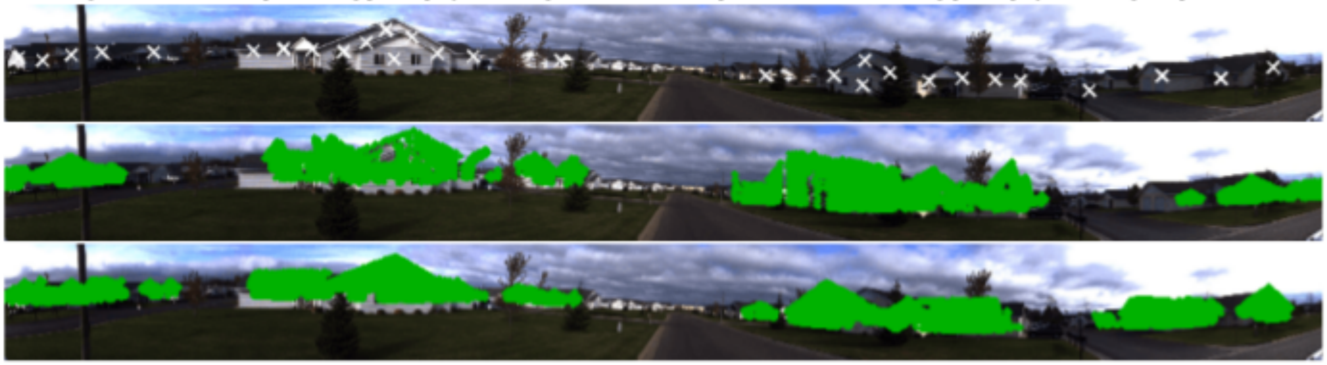

(c) Image 3: 2D features (top), building points projected using RANSAC camera pose (middle) and building points projected using our pose (bottom).

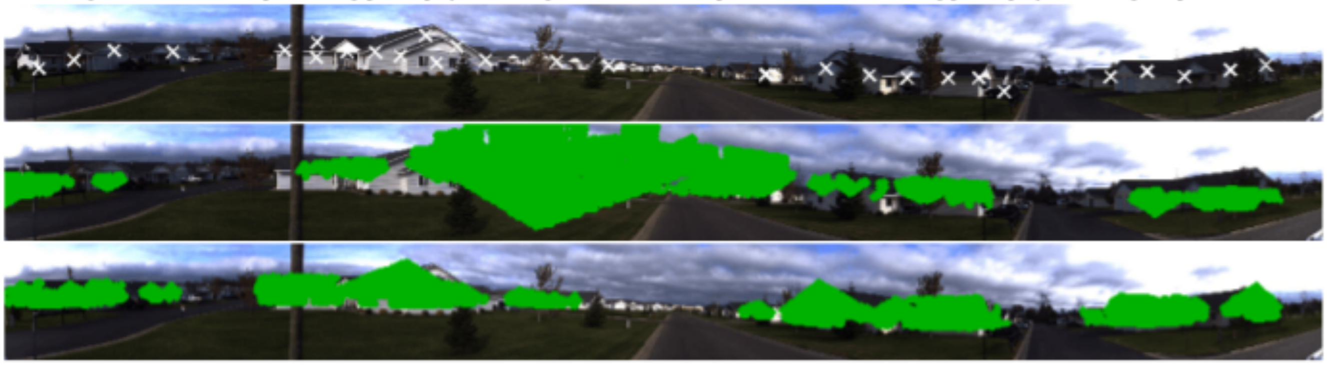

(d) Image 4: 2D features (top), building points projected using RANSAC camera pose (middle) and building points projected using our pose (bottom).

Figure G.5. Qualitative results for 4 test images. Our method (GOPAC) found the correct camera pose for every image.

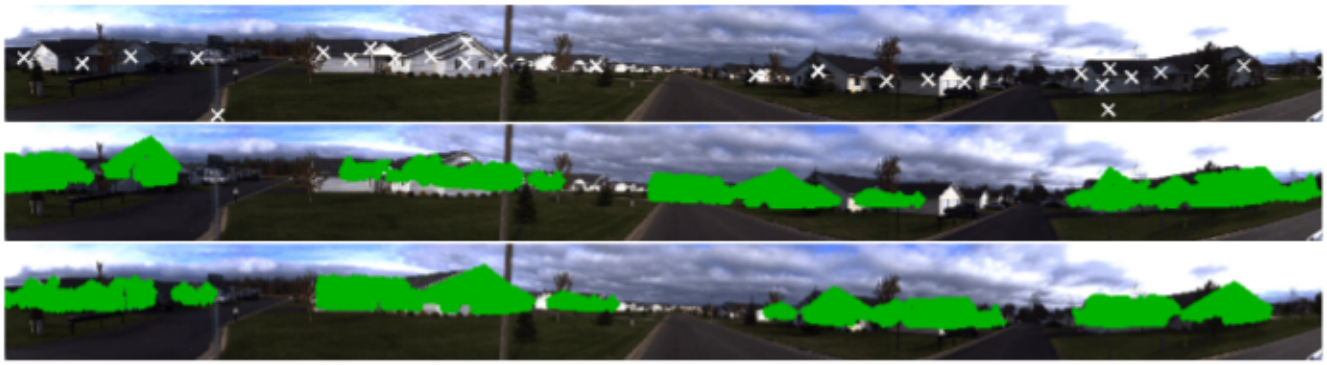

(a) Image 5: 2D features (top), building points projected using RANSAC camera pose (middle) and building points projected using our pose (bottom).

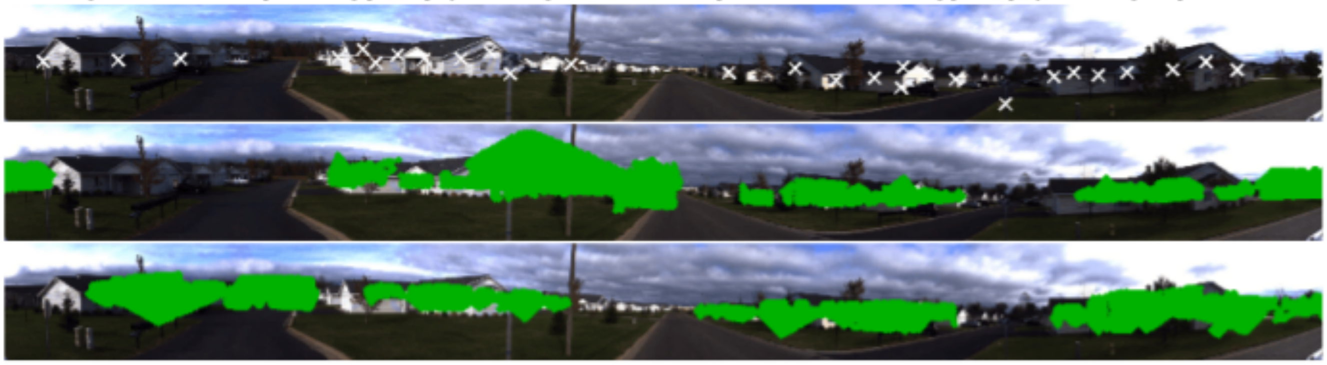

(b) Image 6: 2D features (top), building points projected using RANSAC camera pose (middle) and building points projected using our pose (bottom).

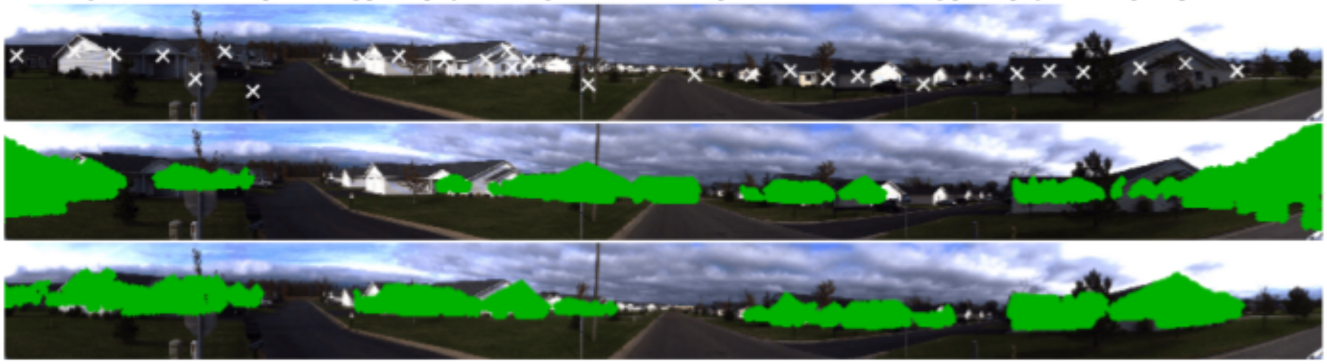

(c) Image 7: 2D features (top), building points projected using RANSAC camera pose (middle) and building points projected using our pose (bottom).

Figure G.6. Qualitative results for 3 test images. Image 6 was a failure case for our method, with respect to camera pose, although it still found the optimal number of inliers. It can be seen that three 2D features were extracted at non-building locations, due to an error in the segmentation. This may have contributed to the algorithm finding an incorrect pose.

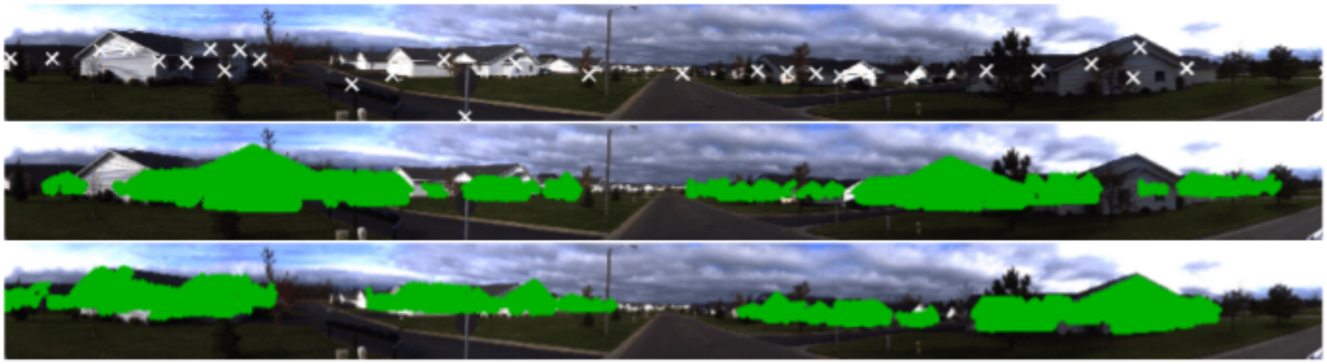

(a) Image 8: 2D features (top), building points projected using RANSAC camera pose (middle) and building points projected using our pose (bottom).

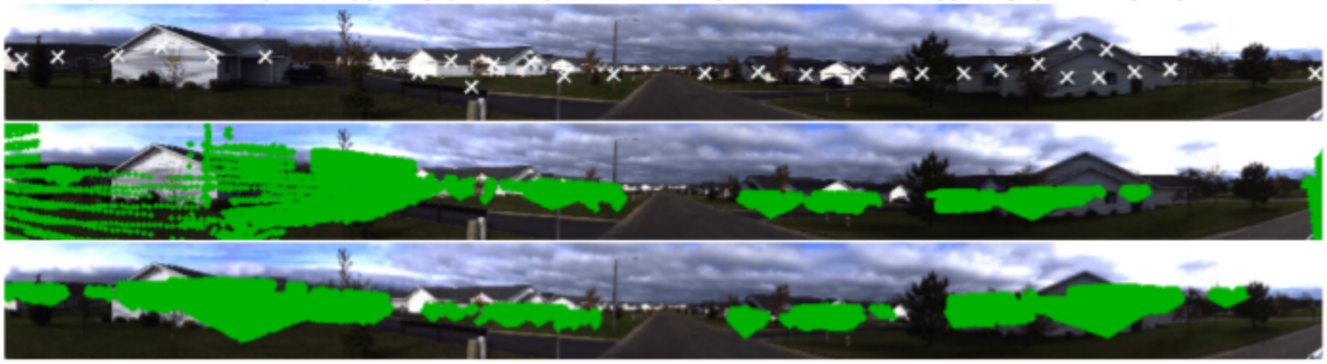

(b) Image 9: 2D features (top), building points projected using RANSAC camera pose (middle) and building points projected using our pose (bottom).

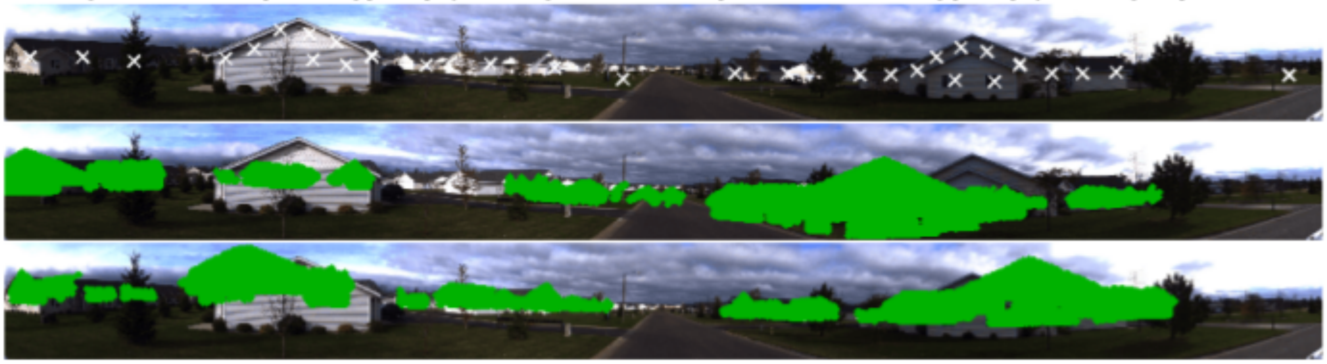

(c) Image 11: 2D features (top), building points projected using RANSAC camera pose (middle) and building points projected using our pose (bottom).

Figure G.7. Qualitative results for 3 test images. Image 9 was a failure case for our method, with respect to camera pose, although it still found the optimal number of inliers. Like the previous failure case, 2D features were extracted at non-building locations, due to an error in the segmentation. This may have contributed to the algorithm finding an incorrect pose.
